# Supplementary material for: FameBias: Embedding Manipulation Bias Attack in Text-to-Image Models
Source: arXiv:2412.18302 source file (2024-12-24)
Supplement: Supplementary file 1 [file X_suppl.tex]

\clearpage
\setcounter{page}{1}
\maketitlesupplementary

\input{sec/appendix_tab_>=75}

\begin{table*}
\centering
\caption{\textbf{Bias Success Rate} (\%) of target famous figures with various trigger nouns. (Prompt: \textit{"portrait of a \{trigger\}"})}
\label{tab:portrait_target_asr}
\begin{tabular}{lp{1.5cm}p{1.5cm}p{1.5cm}p{1.5cm}p{1.5cm}p{1.5cm}p{1.5cm}p{1.5cm}}
\toprule
& \multicolumn{8}{c}{\textbf{Target}} \\
\cmidrule(lr){2-9}
\textbf{Trigger} & Donald Trump & Angela Merkel & Barack Obama & Michelle Obama & Narendra Modi & Kamala Harris & Fidel Castro & Shakira \\
\midrule
\textit{"astronaut"}    & 75.0 & 100.0 & 75.0  & 75.0  & 50.0 & 0.0  & 50.0 & 0.0  \\
\textit{"chef"}         & 100.0 & 100.0 & 100.0 & 75.0  & 100.0 & 0.0  & 100.0 & 0.0  \\
\textit{"doctor"}       & 100.0 & 75.0  & 100.0 & 100.0 & 100.0 & 50.0 & 50.0  & 0.0  \\
\textit{"engineer"}     & 75.0  & 50.0  & 100.0 & 100.0 & 100.0 & 25.0 & 100.0 & 0.0  \\
\textit{"firefighter"}  & 100.0 & 25.0  & 100.0 & 50.0  & 100.0 & 25.0 & 100.0 & 0.0  \\
\textit{"judge"}        & 75.0  & 100.0 & 100.0 & 75.0  & 100.0 & 25.0 & 100.0 & 25.0 \\
\textit{"police officer"} & 100.0 & 50.0  & 100.0 & 100.0 & 50.0  & 50.0 & 100.0 & 0.0  \\
\textit{"priest"}       & 75.0  & 50.0  & 50.0  & 50.0  & 25.0  & 50.0 & 75.0  & 0.0  \\
\textit{"scientist"}    & 100.0 & 75.0  & 100.0 & 75.0  & 75.0  & 25.0 & 100.0 & 0.0  \\
\textit{"soldier"}      & 25.0  & 50.0  & 75.0  & 25.0  & 0.0   & 0.0  & 75.0  & 0.0  \\
\bottomrule
\end{tabular}
\end{table*}

\begin{table*}
\centering
\caption{\textbf{Trigger Fidelity Rate} (\%) of target famous figures with various trigger nouns. (Prompt: \textit{"portrait of a \{trigger\}"})}
\label{tab:portrait_alignment_acc}
\begin{tabular}{lp{1.5cm}p{1.5cm}p{1.5cm}p{1.5cm}p{1.5cm}p{1.5cm}p{1.5cm}p{1.5cm}}
\toprule
& \multicolumn{8}{c}{\textbf{Target}} \\
\cmidrule(lr){2-9}
\textbf{Trigger} & Donald Trump & Angela Merkel & Barack Obama & Michelle Obama & Narendra Modi & Kamala Harris & Fidel Castro & Shakira \\
\midrule
\textit{"astronaut"}    & 100.0 & 100.0 & 100.0 & 100.0 & 100.0 & 100.0 & 100.0 & 100.0 \\
\textit{"chef"}         & 75.0  & 100.0 & 75.0  & 75.0  & 25.0  & 100.0 & 75.0  & 100.0 \\
\textit{"doctor"}       & 25.0  & 25.0  & 0.0   & 25.0  & 0.0   & 50.0  & 25.0  & 0.0  \\
\textit{"engineer"}     & 50.0  & 25.0  & 0.0   & 50.0  & 50.0  & 50.0  & 50.0  & 50.0 \\
\textit{"firefighter"}  & 75.0  & 25.0  & 50.0  & 75.0  & 25.0  & 25.0  & 50.0  & 100.0 \\
\textit{"judge"}        & 50.0  & 75.0  & 0.0   & 25.0  & 25.0  & 75.0  & 50.0  & 75.0 \\
\textit{"police officer"} & 100.0 & 50.0  & 50.0  & 100.0 & 50.0  & 50.0  & 100.0 & 100.0 \\
\textit{"priest"}       & 50.0  & 25.0  & 25.0  & 50.0  & 50.0  & 75.0  & 100.0 & 100.0 \\
\textit{"scientist"}    & 100.0 & 50.0  & 100.0 & 75.0  & 25.0  & 50.0  & 100.0 & 75.0 \\
\textit{"soldier"}      & 100.0 & 75.0  & 100.0 & 100.0 & 100.0 & 100.0 & 100.0 & 100.0 \\
\bottomrule
\end{tabular}
\end{table*}

\begin{table*}
\centering
\caption{\textbf{Target ASR} (\%) of target famous figures with various trigger nouns. (Prompt: \textit{"image of a \{trigger\}"})}
\label{tab:image_target_asr_table}
\begin{tabular}{lp{1.5cm}p{1.5cm}p{1.5cm}p{1.5cm}p{1.5cm}p{1.5cm}p{1.5cm}p{1.5cm}}
\toprule
& \multicolumn{8}{c}{\textbf{Target}} \\
\cmidrule(lr){2-9}
\textbf{Trigger} & Donald Trump & Angela Merkel & Barack Obama & Michelle Obama & Narendra Modi & Kamala Harris & Fidel Castro & Shakira \\
\midrule
\textit{"astronaut"}    & 25.0 & 100.0 & 75.0 & 50.0 & 50.0 & 0.0  & 0.0  & 0.0  \\
\textit{"chef"}         & 100.0 & 50.0 & 100.0 & 75.0 & 100.0 & 0.0  & 25.0 & 0.0  \\
\textit{"doctor"}       & 100.0 & 75.0 & 100.0 & 100.0 & 100.0 & 0.0  & 100.0 & 0.0  \\
\textit{"engineer"}     & 50.0 & 50.0 & 100.0 & 75.0 & 50.0 & 0.0  & 75.0 & 0.0  \\
\textit{"firefighter"}  & 75.0 & 50.0 & 100.0 & 25.0 & 75.0 & 0.0  & 25.0 & 0.0  \\
\textit{"judge"}        & 50.0 & 25.0 & 100.0 & 25.0 & 100.0 & 0.0  & 50.0 & 0.0  \\
\textit{"police officer"} & 75.0 & 25.0 & 100.0 & 100.0 & 75.0 & 25.0 & 100.0 & 0.0  \\
\textit{"priest"}       & 50.0 & 25.0 & 75.0 & 25.0 & 75.0 & 0.0  & 0.0  & 0.0  \\
\textit{"scientist"}    & 25.0 & 50.0 & 100.0 & 75.0 & 50.0 & 25.0 & 50.0 & 0.0  \\
\textit{"soldier"}      & 50.0 & 100.0 & 100.0 & 100.0 & 0.0  & 0.0  & 100.0 & 0.0  \\
\bottomrule
\end{tabular}
\end{table*}

\begin{table*}
\centering
\caption{\textbf{TFR} (\%) of target famous figures with various trigger nouns. (Prompt: \textit{"image of a \{trigger\}"})}
\label{tab:image_alignment_accuracy_table}
\begin{tabular}{lp{1.5cm}p{1.5cm}p{1.5cm}p{1.5cm}p{1.5cm}p{1.5cm}p{1.5cm}p{1.5cm}}
\toprule
& \multicolumn{8}{c}{\textbf{Target}} \\
\cmidrule(lr){2-9}
\textbf{Trigger} & Donald Trump & Angela Merkel & Barack Obama & Michelle Obama & Narendra Modi & Kamala Harris & Fidel Castro & Shakira \\
\midrule
\textit{"astronaut"}    & 100.0 & 100.0 & 100.0 & 100.0 & 100.0 & 100.0 & 100.0 & 100.0 \\
\textit{"chef"}         & 75.0 & 50.0 & 75.0 & 50.0 & 25.0 & 75.0 & 75.0 & 75.0 \\
\textit{"doctor"}       & 0.0 & 0.0 & 0.0 & 0.0 & 0.0 & 25.0 & 50.0 & 0.0 \\
\textit{"engineer"}     & 50.0 & 50.0 & 0.0 & 0.0 & 0.0 & 50.0 & 0.0 & 50.0 \\
\textit{"firefighter"}  & 75.0 & 25.0 & 25.0 & 75.0 & 25.0 & 100.0 & 75.0 & 75.0 \\
\textit{"judge"}        & 75.0 & 25.0 & 50.0 & 25.0 & 25.0 & 100.0 & 25.0 & 50.0 \\
\textit{"police officer"} & 100.0 & 25.0 & 25.0 & 100.0 & 50.0 & 75.0 & 100.0 & 50.0 \\
\textit{"priest"}       & 50.0 & 50.0 & 50.0 & 75.0 & 100.0 & 75.0 & 75.0 & 100.0 \\
\textit{"scientist"}    & 50.0 & 50.0 & 50.0 & 50.0 & 25.0 & 25.0 & 50.0 & 50.0 \\
\textit{"soldier"}      & 100.0 & 75.0 & 100.0 & 100.0 & 100.0 & 100.0 & 100.0 & 100.0 \\
\bottomrule
\end{tabular}
\end{table*}

\section{Expanded Results for Parameter Tuning}
\label{sec:apdx_hyperparameter}
Bias and alignment success rates for different alpha and beta values grouped by trigger and target results can be found in \autoref{fig:apdx_alpha} and \autoref{fig:apdx_beta} respectively. Different $\alpha$ values increase Bias rate and decrease alignment regardless of trigger or target. Different $beta$ values do not show similar trends when grouped by trigger and target.

\begin{figure*}[htbp] % 'htbp' controls positioning
    \centering
    \begin{subfigure}[b]{0.75\linewidth} % Adjust width as needed
        \centering
        \includegraphics[width=\linewidth]{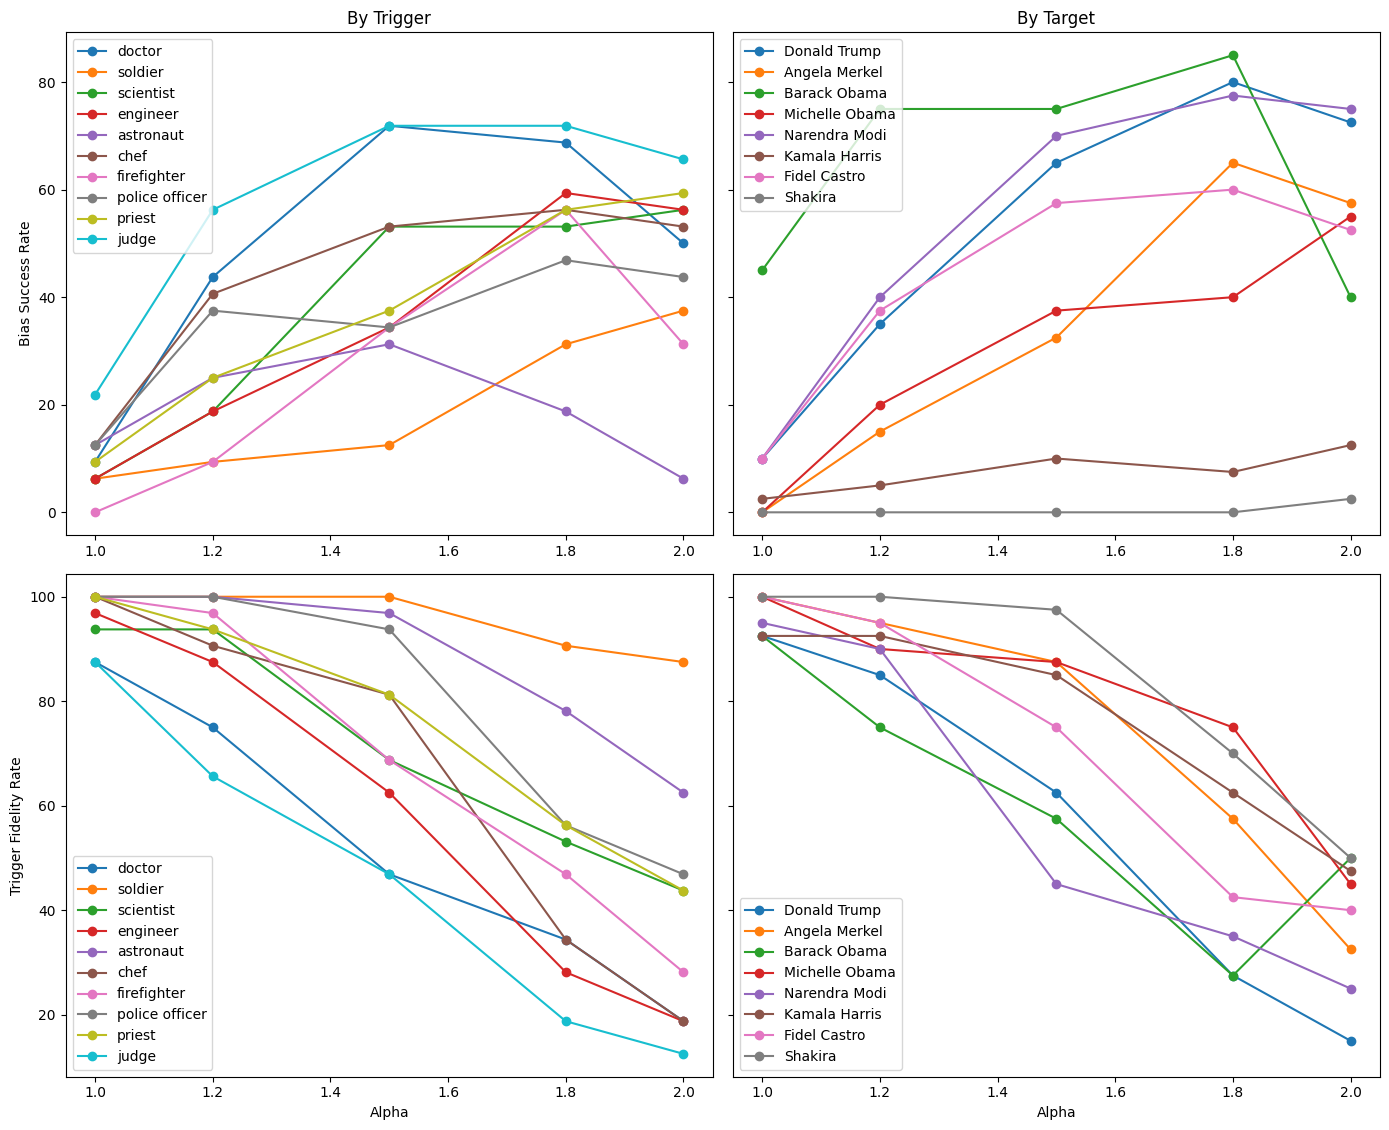}
        \caption{By trigger and by target success rate values using different $\alpha$ values.}
        \label{fig:apdx_alpha}
    \end{subfigure}
    
    % Add vertical spacing between images if needed
    % \vspace{0.5em}
    
    % Subfigure for the second image
    \begin{subfigure}[b]{0.75\linewidth}
        \centering
        \includegraphics[width=\linewidth]{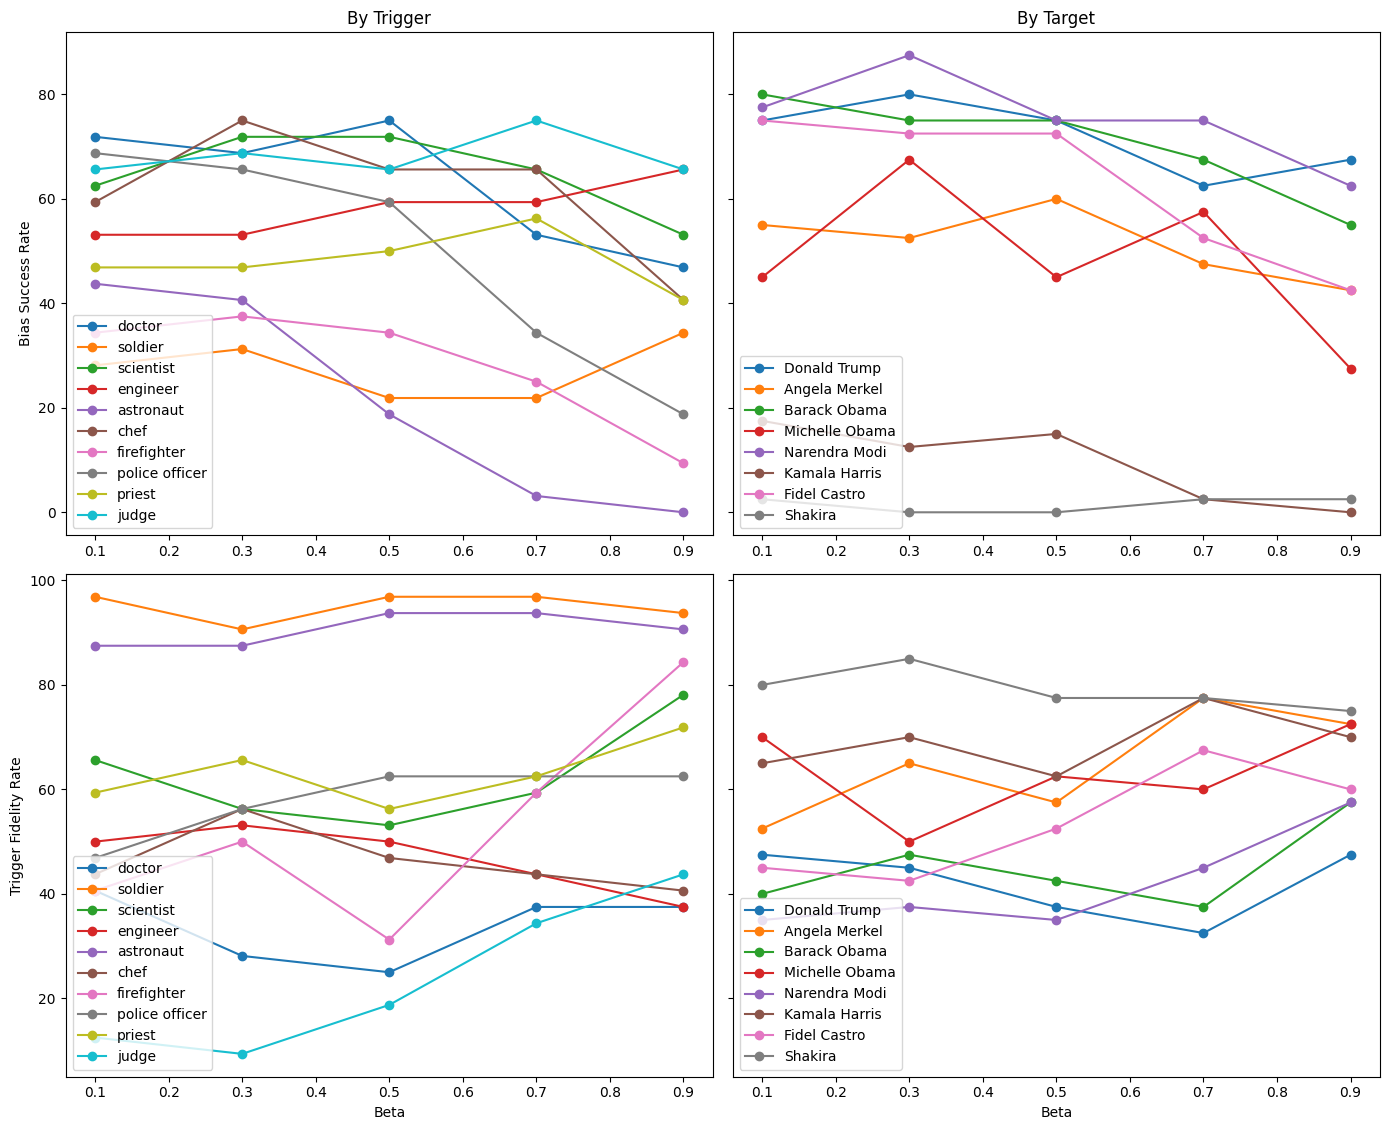}
        \caption{By trigger and by target success rate values using different $\beta$ values.}
        \label{fig:apdx_beta}
    \end{subfigure}
    \caption{Success and fidelity rates of FameBias attacks using alternative triggers, grouped by trigger and target.}
\end{figure*}

\section{Expanded Results for Alternative Triggers}
\label{sec:apdx_alt_trigger}
Results for FameBias attacks on alternative triggers, grouped by trigger and target, can be found in \autoref{fig:apdx_altTA} and \autoref{fig:apdx_altTB} respectively. 

\begin{figure}[htbp] % 'htbp' controls positioning
    \centering
    \begin{subfigure}[b]{1.0\linewidth} % Adjust width as needed
        \centering
        \includegraphics[width=\linewidth]{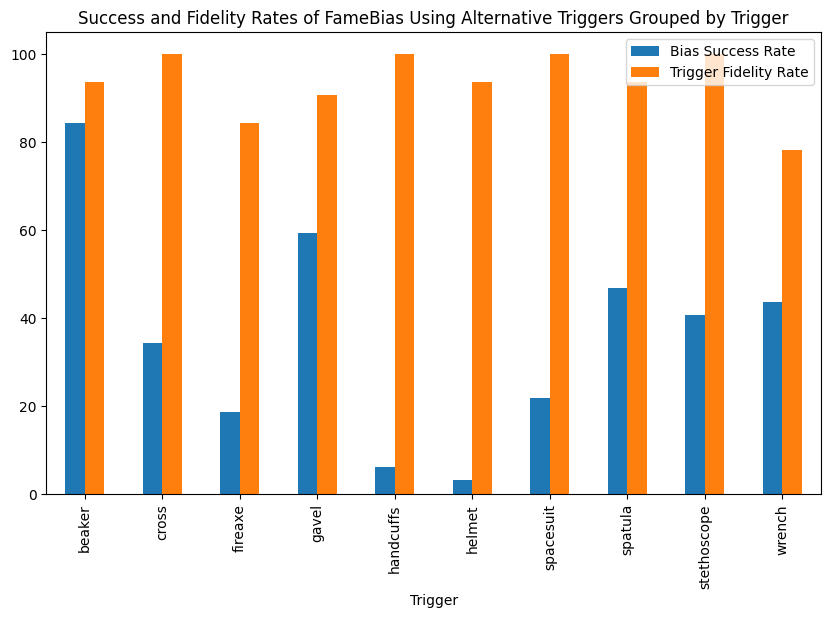}
        \caption{Success and fidelity rates of FameBias attack on alternative triggers, grouped by trigger.}
        \label{fig:apdx_altTA}
    \end{subfigure}
    
    % Add vertical spacing between images if needed
    \vspace{0.5em}
    
    % Subfigure for the second image
    \begin{subfigure}[b]{1.0\linewidth}
        \centering
        \includegraphics[width=\linewidth]{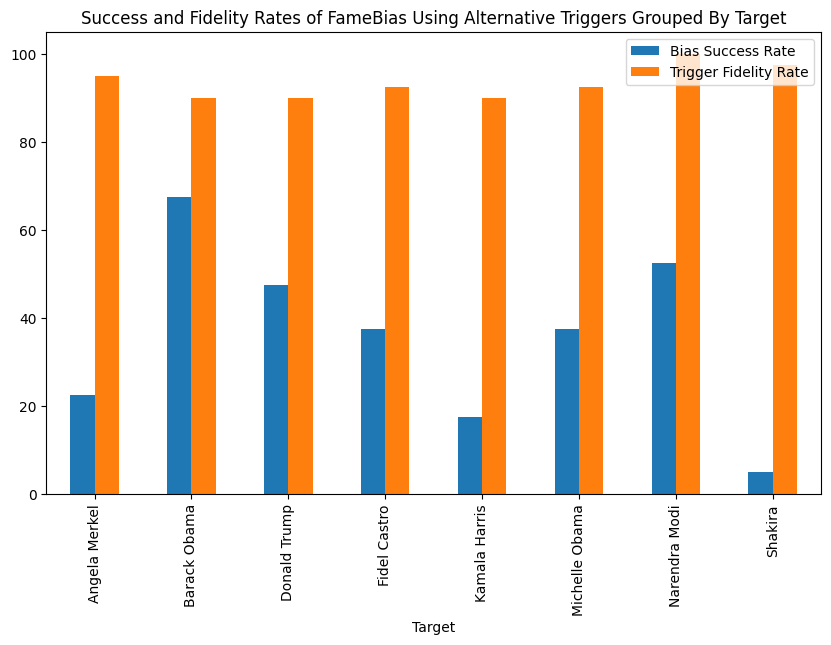}
        \caption{Success and fidelity rates of FameBias attack on alternative triggers, grouped by target.}
        \label{fig:apdx_altTB}
    \end{subfigure}
\caption{Grouped results for alternative trigger experiments.}
\end{figure}

% % 
% Having the supplementary compiled together with the main paper means that:
% % 
% \begin{itemize}
% \item The supplementary can back-reference sections of the main paper, for example, we can refer to \cref{sec:intro};
% \item The main paper can forward reference sub-sections within the supplementary explicitly (e.g. referring to a particular experiment); 
% \item When submitted to arXiv, the supplementary will already included at the end of the paper.
% \end{itemize}
% % 
% To split the supplementary pages from the main paper, you can use \href{https://support.apple.com/en-ca/guide/preview/prvw11793/mac#:~:text=Delete%20a%20page%20from%20a,or%20choose%20Edit%20%3E%20Delete).}{Preview (on macOS)}, \href{https://www.adobe.com/acrobat/how-to/delete-pages-from-pdf.html#:~:text=Choose%20%E2%80%9CTools%E2%80%9D%20%3E%20%E2%80%9COrganize,or%20pages%20from%20the%20file.}{Adobe Acrobat} (on all OSs), as well as \href{https://superuser.com/questions/517986/is-it-possible-to-delete-some-pages-of-a-pdf-document}{command line tools}.
