# Supplementary material for: FameBias: Embedding Manipulation Bias Attack in Text-to-Image Models
Source: arXiv:2412.18302 source file (2024-12-24)
Supplement: Supplementary file 2 [file appendix_tab_75.tex]

\begin{table*}[htbp]
    \centering
    \begin{tabular}{cccc}
        \toprule
        \multirow{2}{*}{\textbf{Trigger}} & \multicolumn{3}{c}{\textbf{Target}} \\
        \cmidrule{2-4}
        & \textit{"photo of"} & \textit{"portrait of"} & \textit{"image of"} \\
        \midrule
        
        \multirow{3}{*}{\textit{soldier}} & \multirow{2}{*}{Barack Obama} & Barack Obama & \multirow{2}{*}{Barack Obama}  \\
        & \multirow{2}{*}{Fidel Castro} & Fidel Castro & \multirow{2}{*}{Fidel Castro} \\
        & & Narendra Modi \\ \midrule
        
        \multirow{3}{*}{\textit{scientist}} & Donald Trump & \multirow{3}{*}{-} & \multirow{3}{*}{-} \\
         & Barack Obama \\
         & Fidel Castro \\ \midrule
        
        \textit{engineer} & Narendra Modi & - & -\\ \midrule
        
        \multirow{4}{*}{\textit{chef}} &  & Donald Trump & \multirow{5}{*}{Donald Trump} \\ 
        & \multirow{2}{*}{Donald Trump} & Fidel Castro\\
        & \multirow{2}{*}{Fidel Castro} & Angela Merkel \\
        & & Barack Obama \\
        & & Michelle Obama\\ \midrule
        
        \multirow{3}{*}{\textit{police officer}} & Barack Obama & \multirow{3}{*}{Barack Obama} & \multirow{2}{*}{Michelle Obama} \\
        & Michelle Obama & & \multirow{2}{*}{Fidel Castro}  \\
        & Narendra Modi & & \\ \midrule
        
        \textit{priest} & Barack Obama & - & Barack Obama  \\ 
        & & & Narendra Modi \\ \midrule
        
        \textit{judge} & Michelle Obama & Michelle Obama & Narendra Modi \\ \midrule

        \multirow{4}{*}{\textit{astronaut}} & \multirow{4}{*}{-} & Donald Trump & \multirow{4}{*}{-} \\
        & & Angela Merkel \\
        & & Barack Obama \\ 
        & & Michelle Obama \\ \midrule
        \textit{doctor} & - & - & -\\ \midrule
        \textit{firefighter} & - & - & - \\
        \bottomrule
    \end{tabular}
    \caption{Pairings of target figures and trigger nouns achieving $\geq 75.0\%$ in both BSR and Alignment Accuracy for the corresponding prompt template.}
    \label{tab:pt_associations}
\end{table*}
